# Supplementary material for: Auditing Frameworks Need Resource Isolation: A Systematic Study on the Super Producer Threat to System Auditing and Its Mitigation
Source: arXiv:2307.15895 source file (2023-07-29)
Supplement: Supplementary file 1 [file appendix.tex]

\section{APPENDIX}
\subsection{More Graphs for \S~\ref{ssec:eventdrop}}
\label{app:eventdrop}
\begin{figure*}
    \centering
    \includegraphics[width=\textwidth]{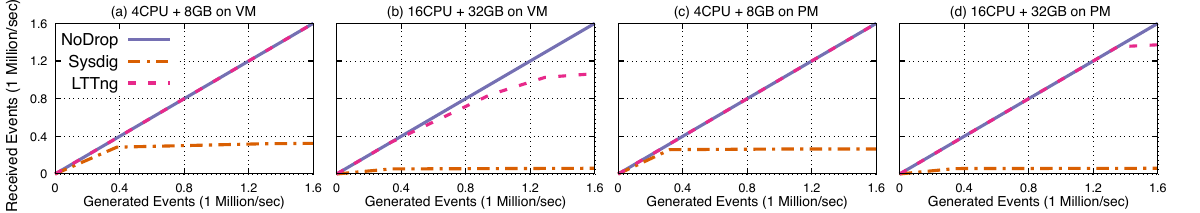}
    \vspace{-0.25in}
    \caption{The number of events dropped by \toolname and baselines with different hardware configurations. The x-axis is the number of generated events in 30 seconds, the y-axis is the number of events handled by the auditing framework.}
    \label{fig:drop}
\end{figure*}
Figure~\ref{fig:drop} shows how existing auditing frameworks drop events with different hardware configurations other than those in Section~\ref{ssec:eventdrop}. It also shows that \toolname does not drop any events. This result is consistent with the conclusion in Section~\ref{ssec:eventdrop}.

\subsection{More Graphs for \S~\ref{ssec:slowdonw}}
\label{app:isolation}

\begin{figure*}
\vspace{-0.07in}
    \centering
    \includegraphics[width=\textwidth]{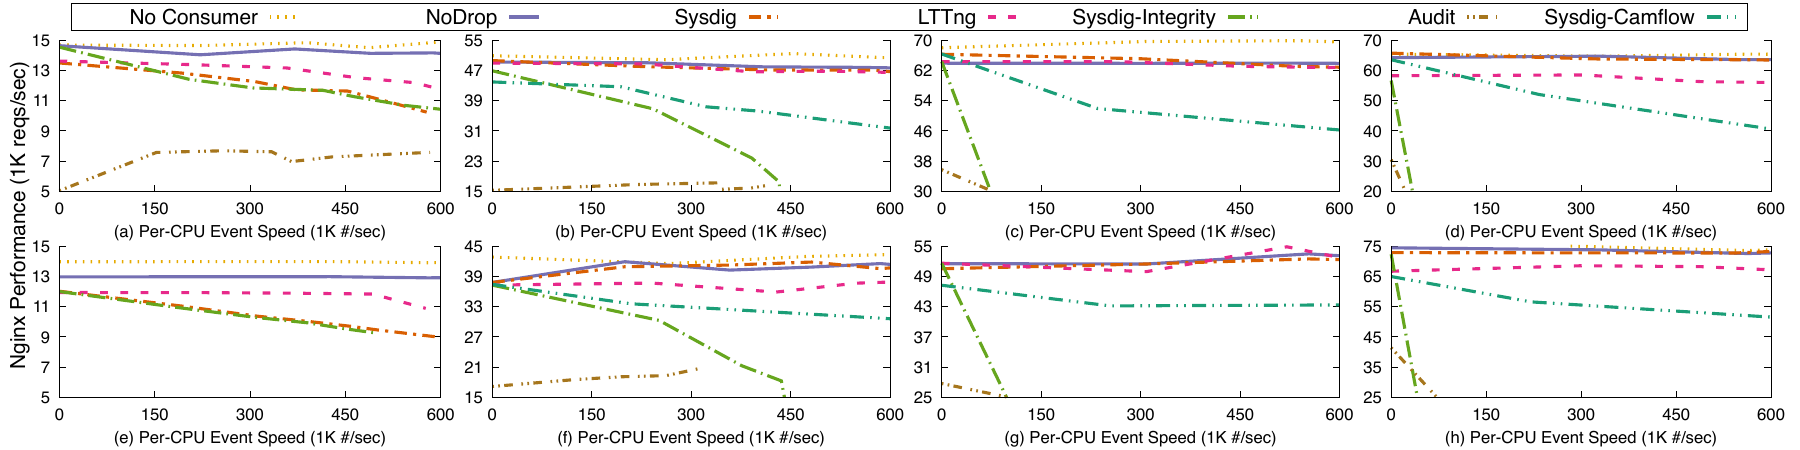}
    \caption{The performance of Nginx on different platforms with different workloads from the super-producer on platforms with different hardware configurations. The x-axis is the speed of generated events in 30 seconds,  thy-axis is the performance score of Nginx, measured in the number of requests per second.}
    \label{fig:rq12-nginx}
\end{figure*}

\begin{figure*}
\vspace{-0.07in}
    \centering
    \includegraphics[width=\textwidth]{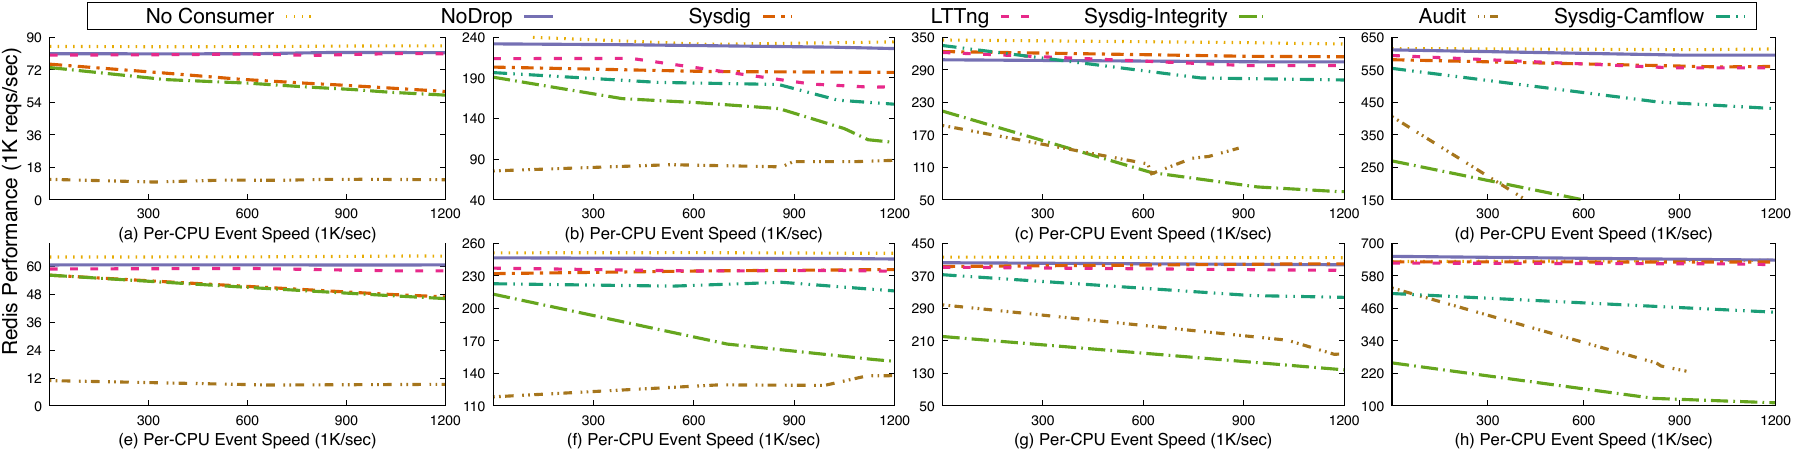}
    \caption{The performance of Redis on different platforms with different workloads from the super-producer on  platforms with different hardware configurations. The x-axis is the speed of generated events in 30 seconds,  the y-axis is the performance score of Redis, measured in the bandwidth.}
    \label{fig:rq12-redis}
\end{figure*}

\begin{figure*}
\vspace{-0.07in}
    \centering
    \includegraphics[width=\textwidth]{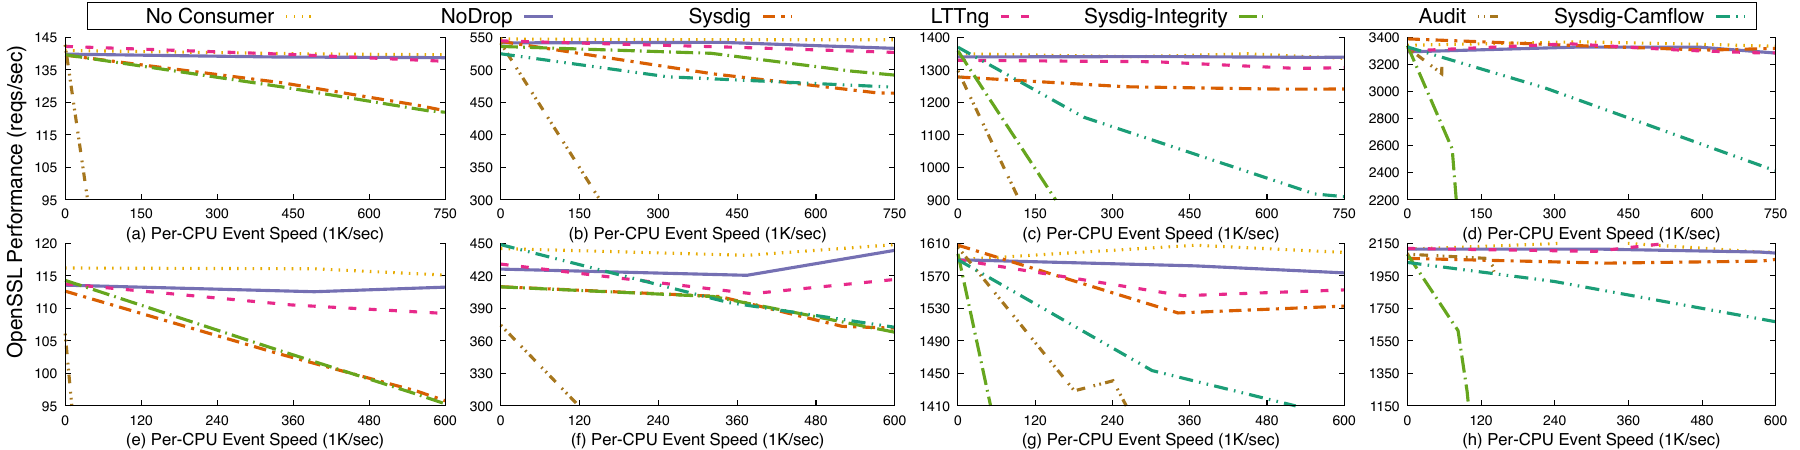}
    \caption{The performance of OpenSSL on different platforms with different workloads from the super-producer on  platforms with different hardware configurations. The x-axis is the speed of generated events in 30 seconds, the y-axis is the performance score of OpenSSL, measured in the number of requests per second.}
    \label{fig:rq12-openssl}
\end{figure*}

Figure~\ref{fig:rq12-nginx}, Figure~\ref{fig:rq12-redis} and Figure~\ref{fig:rq12-openssl} show the Nginx, Redis, and OpenSSL results respectively. Note that for all three figures, subfigure (a)-(h) represent configurations of 1 CPU core with 2GB memory, 4 CPU cores with 8GB memory, 16 CPU cores with 32GB memory, and 32 CPU cores with 64 GB memory on both virtual and physical machine respectively. Overall, existing auditing frameworks can substantially slow down other applications when the super producer's workload increases. The Figures also show that \toolname does not slow other applications. These results are consistent with the conclusion in Section~\ref{ssec:slowdonw}.

\subsection{More Results for \S~\ref{ssec:syscallovehead}}
\label{app:syscallovehead}
Table~\ref{tab:benchmark} shows the performance scores of \code{lmbench} for other hardware configurations besides those in \S~\ref{ssec:syscallovehead}. Overall, the conclusion is consistent with \S~\ref{ssec:syscallovehead}.

\begin{table}[h]
    \centering
    \caption{\label{tab:lmbench2} Performance scores of \code{lmbench}. \emph{Values are shown as percentages relative to Sysdig. The negative value means \toolname is faster than Sysdig.}}
    \resizebox{0.5\textwidth}{!}{
    \begin{tabular}{lrrrrr}
    \toprule
Configurations & 
    C1 & C2 & C3 & C4 & Ave  \\ 
    \cmidrule{1-6}
    \multicolumn{6}{c}{\small Syscall Tests} \\
    \cmidrule{0-1}\cmidrule{2-6}
NULL syscall & 
    -11.2\% & -18.0\% & -13.2\% & -8.1\% & -12.6\% \\ 
stat & 
    -4.4\% & +9.1\% & -0.0\% & +1.2\% & -3.1\% \\
fstat & 
    +5.4\% & +4.0\% & -1.2\% & +3.2\% & +2.9\% \\ 
open/close file & 
    -0.5\% & -8.0\% & -0.9\% & -3.0\% & -3.1\% \\ 
read file & 
    -0.5\% & +3.0\% & +5.9\% & +5.9\% & +3.6\% \\ 
write file & 
    +1.5\% & +2.7\% & +6.0\% & +6.9\% & +4.3\% \\ 
    \cmidrule{0-1}\cmidrule{2-6}
    \multicolumn{6}{c}{\small File Access} \\
    \cmidrule{0-1}\cmidrule{2-6}
file create (0K) & 
    +2.1\% & +7.6\% & -0.7\% & +0.3\% & +2.4\% \\ 
file delete (0K) & 
    -2.5\% & -2.0\% & -0.5\% & 0.0\% & -1.3\% \\ 
file create (10K) & 
    -4.4\% & +1.6\% & -1.2\% & -1.2\% & -1.3\% \\ 
file delete (10K) & 
    -4.1\% & -2.9\% & -0.3\% & +0.2\% & -1.8\% \\ 
pipe & 
    +0.5\% & -3.8\% & +7.0\% & +7.0\% & +2.7\% \\ 
AF\_UNIX & 
    -6.3\% & -8.6\% & +8.5\% & +9.0\% & +0.6\% \\ 
    \bottomrule
    \end{tabular}
    }
    \label{tab:benchmark}
\end{table}

\subsection{More Results for \S~\ref{sec:appoverhead}}
\label{app:overhead}
Table~\ref{tab:benchmarkidle2} and Table~\ref{tab:benchmarkbusy2} show the application benchmark results for other hardware configurations besides those in \S~\ref{sec:appoverhead}. On average, the application overhead of \toolname is smaller than that of Sysdig. The conclusion in this section is also consistent with the conclusion in \S~\ref{sec:appoverhead}.

\begin{table*}[!ht]
\centering
\label{tab:new2}
\begin{subtable}{0.45\textwidth}
\centering
\caption{\textbf{Benchmark WITHOUT super producer.}}
\label{tab:benchmarkidle2}
    \begin{tabular}{l|l|rrrr} 
\hline
\textbf{Application} & \textbf{Collector}                                & \textbf{C2}                                                 & \textbf{C3}                                                 & \textbf{C6}                                                  & \textbf{C7}                                                  \\ 
\hline\hline
\multirow{3}{*}{Nginx}           & Nodrop                                   & 5.00                                               & 2.40                                               & 8.84                                                & 3.37                                                \\
                                 & Sysdig                                   & 16.30                                              & 12.10                                              & 21.20                                               & 9.50                                                \\ 
\cline{2-6}
                                 & {\cellcolor[rgb]{0.906,0.906,0.906}}DIFF & {\cellcolor[rgb]{0.906,0.906,0.906}}\textbf{-9.70} & {\cellcolor[rgb]{0.906,0.906,0.906}}\textbf{-8.60} & {\cellcolor[rgb]{0.906,0.906,0.906}}\textbf{-10.20} & {\cellcolor[rgb]{0.906,0.906,0.906}}\textbf{-5.60}  \\ 
\hline
\multirow{3}{*}{Redis}           & Nodrop                                   & 6.40                                               & 7.40                                               & 4.18                                                & 11.79                                               \\
                                 & Sysdig                                   & 14.10                                              & 13.50                                              & 16.40                                               & 15.60                                               \\ 
\cline{2-6}
                                 & {\cellcolor[rgb]{0.906,0.906,0.906}}DIFF & \textbf{{\cellcolor[rgb]{0.906,0.906,0.906}}-9.00 }         & \textbf{{\cellcolor[rgb]{0.906,0.906,0.906}}-7.10 }         & \textbf{{\cellcolor[rgb]{0.906,0.906,0.906}}-10.50 }         & \textbf{{\cellcolor[rgb]{0.906,0.906,0.906}}-3.30 }          \\ 
\hline
\multirow{3}{*}{Postmark}        & Nodrop                                   & 28.20                                              & 20.20                                              & 35.77                                               & 27.57                                               \\
                                 & Sysdig                                   & 23.20                                              & 18.40                                              & 23.20                                               & 16.50                                               \\ 
\cline{2-6}
                                 & {\cellcolor[rgb]{0.906,0.906,0.906}}DIFF & {\cellcolor[rgb]{0.906,0.906,0.906}}\textbf{4.10}  & {\cellcolor[rgb]{0.906,0.906,0.906}}\textbf{1.50}  & {\cellcolor[rgb]{0.906,0.906,0.906}}\textbf{10.20}  & {\cellcolor[rgb]{0.906,0.906,0.906}}\textbf{9.50}   \\ 
\hline
\multirow{3}{*}{\makecell{Django \\ (Python)}} & Nodrop                                   & 1.60                                               & 1.00                                               & 1.60                                                & 0.50                                                \\
                                 & Sysdig                                   & 1.20                                               & 0.20                                               & 1.40                                                & 0.10                                                \\ 
\cline{2-6}
                                 & {\cellcolor[rgb]{0.906,0.906,0.906}}DIFF & {\cellcolor[rgb]{0.906,0.906,0.906}}0.50           & {\cellcolor[rgb]{0.906,0.906,0.906}}0.80           & {\cellcolor[rgb]{0.906,0.906,0.906}}0.20            & {\cellcolor[rgb]{0.906,0.906,0.906}}0.40            \\ 
\hline
\multirow{3}{*}{\makecell{http \\ (Golang)}}   & Nodrop                                   & 6.20                                               & 2.40                                               & 6.19                                                & 4.20                                                \\
                                 & Sysdig                                   & 10.60                                              & 4.40                                               & 11.90                                               & 4.10                                                \\ 
\cline{2-6}
                                 & {\cellcolor[rgb]{0.906,0.906,0.906}}DIFF & {\cellcolor[rgb]{0.906,0.906,0.906}}\textbf{-4.00} & {\cellcolor[rgb]{0.906,0.906,0.906}}\textbf{-1.80} & {\cellcolor[rgb]{0.906,0.906,0.906}}\textbf{-5.10}  & {\cellcolor[rgb]{0.906,0.906,0.906}}0.10            \\ 
\hline
\multirow{3}{*}{OpenSSL}         & Nodrop                                   & 1.00                                               & 0.10                                               & 0.00                                                & 1.60                                                \\
                                 & Sysdig                                   & 0.40                                               & 0.50                                               & 0.20                                                & 1.70                                                \\ 
\cline{2-6}
                                 & {\cellcolor[rgb]{0.906,0.906,0.906}}DIFF & {\cellcolor[rgb]{0.906,0.906,0.906}}0.60           & {\cellcolor[rgb]{0.906,0.906,0.906}}-0.30          & {\cellcolor[rgb]{0.906,0.906,0.906}}-0.20           & {\cellcolor[rgb]{0.906,0.906,0.906}}-0.10           \\ 
\hline
\multirow{3}{*}{7-ZIP}           & Nodrop                                   & 1.20                                               & 0.40                                               & 0.80                                                & 1.10                                                \\
                                 & Sysdig                                   & 0.70                                               & 0.30                                               & 1.00                                                & 0.80                                                \\ 
\cline{2-6}
                                 & {\cellcolor[rgb]{0.906,0.906,0.906}}DIFF & {\cellcolor[rgb]{0.906,0.906,0.906}}0.50           & {\cellcolor[rgb]{0.906,0.906,0.906}}-0.10          & {\cellcolor[rgb]{0.906,0.906,0.906}}-0.20           & {\cellcolor[rgb]{0.906,0.906,0.906}}0.30            \\ 
\hline
\multirow{3}{*}{PostgreSQL}      & Nodrop                                   & 6.40                                               & 4.72                                               & 8.80                                                & 6.10                                                \\
                                 & Sysdig                                   & 10.70                                              & 8.30                                               & 10.30                                               & 7.80                                                \\ 
\cline{2-6}
                                 & {\cellcolor[rgb]{0.906,0.906,0.906}}DIFF & \textbf{{\cellcolor[rgb]{0.906,0.906,0.906}}-4.04  }        & \textbf{{\cellcolor[rgb]{0.906,0.906,0.906}}-3.40   }       & \textbf{{\cellcolor[rgb]{0.906,0.906,0.906}}-1.30    }       & \textbf{{\cellcolor[rgb]{0.906,0.906,0.906}}-1.60     }      \\
\hline
\end{tabular}
\end{subtable}
\hspace{1cm}
\begin{subtable}{0.45\textwidth}
\centering
\caption{\textbf{Benchmark WITH super producer.}}
\label{tab:benchmarkbusy2}
\begin{tabular}{rrrr} 
\hline
 \textbf{C2}                                & \textbf{C3}                                & \textbf{C6}                                & \textbf{C7}                                \\ 
\hline\hline
5.10                                       & 7.80                                       & 4.34                                       & 7.99                                       \\
                                13.50                                      & 12.76                                      & 10.30                                      & 11.10                                      \\ 
\cline{2-6}
                                \textbf{{\cellcolor[rgb]{0.906,0.906,0.906}}-7.40 }  & \textbf{{\cellcolor[rgb]{0.906,0.906,0.906}}-4.40}   & \textbf{{\cellcolor[rgb]{0.906,0.906,0.906}}-5.40 }  & \textbf{{\cellcolor[rgb]{0.906,0.906,0.906}}-2.80 }  \\ 
\hline
 2.30                                       & 1.30                                       & 1.25                                       & 0.28                                       \\
                    21.07                                      & 8.00                                       & 10.90                                      & 3.70                                       \\ 
\cline{2-6}
                               \textbf{{\cellcolor[rgb]{0.906,0.906,0.906}}-15.50}  & \textbf{{\cellcolor[rgb]{0.906,0.906,0.906}}-6.20}   & \textbf{{\cellcolor[rgb]{0.906,0.906,0.906}}-8.70}    & \textbf{{\cellcolor[rgb]{0.906,0.906,0.906}}-3.30}   \\ 
\hline
22.10                                      & 39.90                                      & 20.30                                      & 35.50                                      \\
                          4.54                                       & 17.66                                      & 8.77                                       & 18.44                                      \\ 
\cline{2-6}
                             \textbf{{\cellcolor[rgb]{0.906,0.906,0.906}}16.80 }  & \textbf{{\cellcolor[rgb]{0.906,0.906,0.906}}18.90}   & \textbf{{\cellcolor[rgb]{0.906,0.906,0.906}}10.60 }  & \textbf{{\cellcolor[rgb]{0.906,0.906,0.906}}14.40 }  \\ 
\hline
 1.50                                       & 1.70                                       & 1.60                                       & 2.20                                       \\
                         3.15                                       & 0.20                                       & 1.80                                       & 1.09                                       \\ 
\cline{2-6}
                                 \textbf{{\cellcolor[rgb]{0.906,0.906,0.906}}-1.60 } & \textbf{{\cellcolor[rgb]{0.906,0.906,0.906}}1.50 }  & {\cellcolor[rgb]{0.906,0.906,0.906}}-0.20  & \textbf{{\cellcolor[rgb]{0.906,0.906,0.906}}1.10}   \\ 
\hline
 3.60                                       & 4.50                                       & 7.30                                       & 4.20                                       \\
                                 2.47                                       & 1.65                                       & 6.45                                       & 1.26                                       \\ 
\cline{2-6}
                        \textbf{{\cellcolor[rgb]{0.906,0.906,0.906}}1.10  } & \textbf{{\cellcolor[rgb]{0.906,0.906,0.906}}2.80 }  & \textbf{{\cellcolor[rgb]{0.906,0.906,0.906}}0.80 }  & \textbf{{\cellcolor[rgb]{0.906,0.906,0.906}}2.90   }\\ 
\hline
 2.60                                       & 0.47                                       & 2.81                                       & 1.35                                       \\
                              21.71                                      & 13.91                                      & 22.10                                      & 9.10                                       \\ 
\cline{2-6}
                              \textbf{{\cellcolor[rgb]{0.906,0.906,0.906}}-15.70 }&  \textbf{{\cellcolor[rgb]{0.906,0.906,0.906}}-11.80 }& \textbf{{\cellcolor[rgb]{0.906,0.906,0.906}}-15.80 }& \textbf{{\cellcolor[rgb]{0.906,0.906,0.906}}-7.10  }\\ 
\hline
 0.90                                       & 1.30                                       & 0.70                                       & 0.90                                       \\
                         16.38                                      & 6.74                                       & 15.22                                      & 6.32                                       \\ 
\cline{2-6}
                               \textbf{{\cellcolor[rgb]{0.906,0.906,0.906}}-13.30 }& \textbf{{\cellcolor[rgb]{0.906,0.906,0.906}}-5.10  }& \textbf{{\cellcolor[rgb]{0.906,0.906,0.906}}-12.60 }& \textbf{{\cellcolor[rgb]{0.906,0.906,0.906}}-5.10  }\\ 
\hline
 9.40                                       & 7.30                                       & 10.70                                      & 8.90                                       \\
                           13.38                                      & 7.94                                       & 13.20                                      & 9.32                                       \\ 
\cline{2-6}
                              \textbf{{\cellcolor[rgb]{0.906,0.906,0.906}}-3.60 } & {\cellcolor[rgb]{0.906,0.906,0.906}}-0.59  & \textbf{{\cellcolor[rgb]{0.906,0.906,0.906}}-2.20}  & {\cellcolor[rgb]{0.906,0.906,0.906}}-0.38  \\
\hline
\end{tabular}
\end{subtable}
\caption{\textbf{We measured the processing time per request/transaction for seven representative applications and a Kubernetes-based PostgreSQL. For each application, the first two lines show the relative runtime overhead (\%) compared to vanilla Linux, where a lower value indicates performance closer to that of vanilla Linux. The third line shows the relative overhead between Nodrop and Sysdig, with values smaller than 0 indicating that \toolname outperforms Sysdig. For brevity, we denote this as DIFF. We report the mean values across 10 runs, with p-values less than 0.05 shown in bold.}}
\end{table*}
